# Supplementary material for: Tracking Summer Greenland Blocking: the Upstream Pathway Shapes Historical Extremes and Future Change
Source: arXiv:2601.02032 source file (2026-06-19)
Supplement: Supplementary file 1 [file supplementary_materials.tex]

\documentclass[12pt,a4paper]{article}

% -------------------------------
% Basic packages
% -------------------------------
\usepackage[T1]{fontenc}
\usepackage[english]{babel}
\usepackage{geometry}
\geometry{margin=1in}
\usepackage{setspace}
\onehalfspacing

\usepackage{graphicx}     % for figures
\usepackage{authblk}      % for authors and affiliations
\usepackage[numbers,sort&compress]{natbib}

\usepackage{hyperref}
\hypersetup{
    colorlinks = true,
    linkcolor  = blue,
    citecolor  = blue,
    urlcolor   = blue
}

% -------------------------------
% Title and authors
% -------------------------------
\title{Supplementary Materials for:\\
\textbf{Tracking Summer Greenland Blocking: the Upstream Pathway Shapes Historical Extremes and Future Change}}

\author[1,2]{Michele Filippucci\thanks{Corresponding author: \href{mailto:michele.filippucci@unitn.it}{michele.filippucci@unitn.it}}}
\author[3]{Jacob Maddison}
\author[1,4]{Simona Bordoni}

\affil[1]{Department of Civil, Environmental and Mechanical Engineering, University of Trento, Trento, Italy}
\affil[2]{Istituto Universitario Superiore di Pavia, Pavia, Italy}
\affil[3]{Department of Mathematics and Statistics, University of Exeter, Exeter, UK}
\affil[4]{Center Agriculture Food Environment (C3A), University of Trento, San Michele all’Adige, Italy}

\date{\today}

% -------------------------------
% Document
% -------------------------------
\begin{document}

\maketitle

\section{Supplementary Figures}

\begin{figure}
    \centering
    \includegraphics[width=0.8\textwidth]{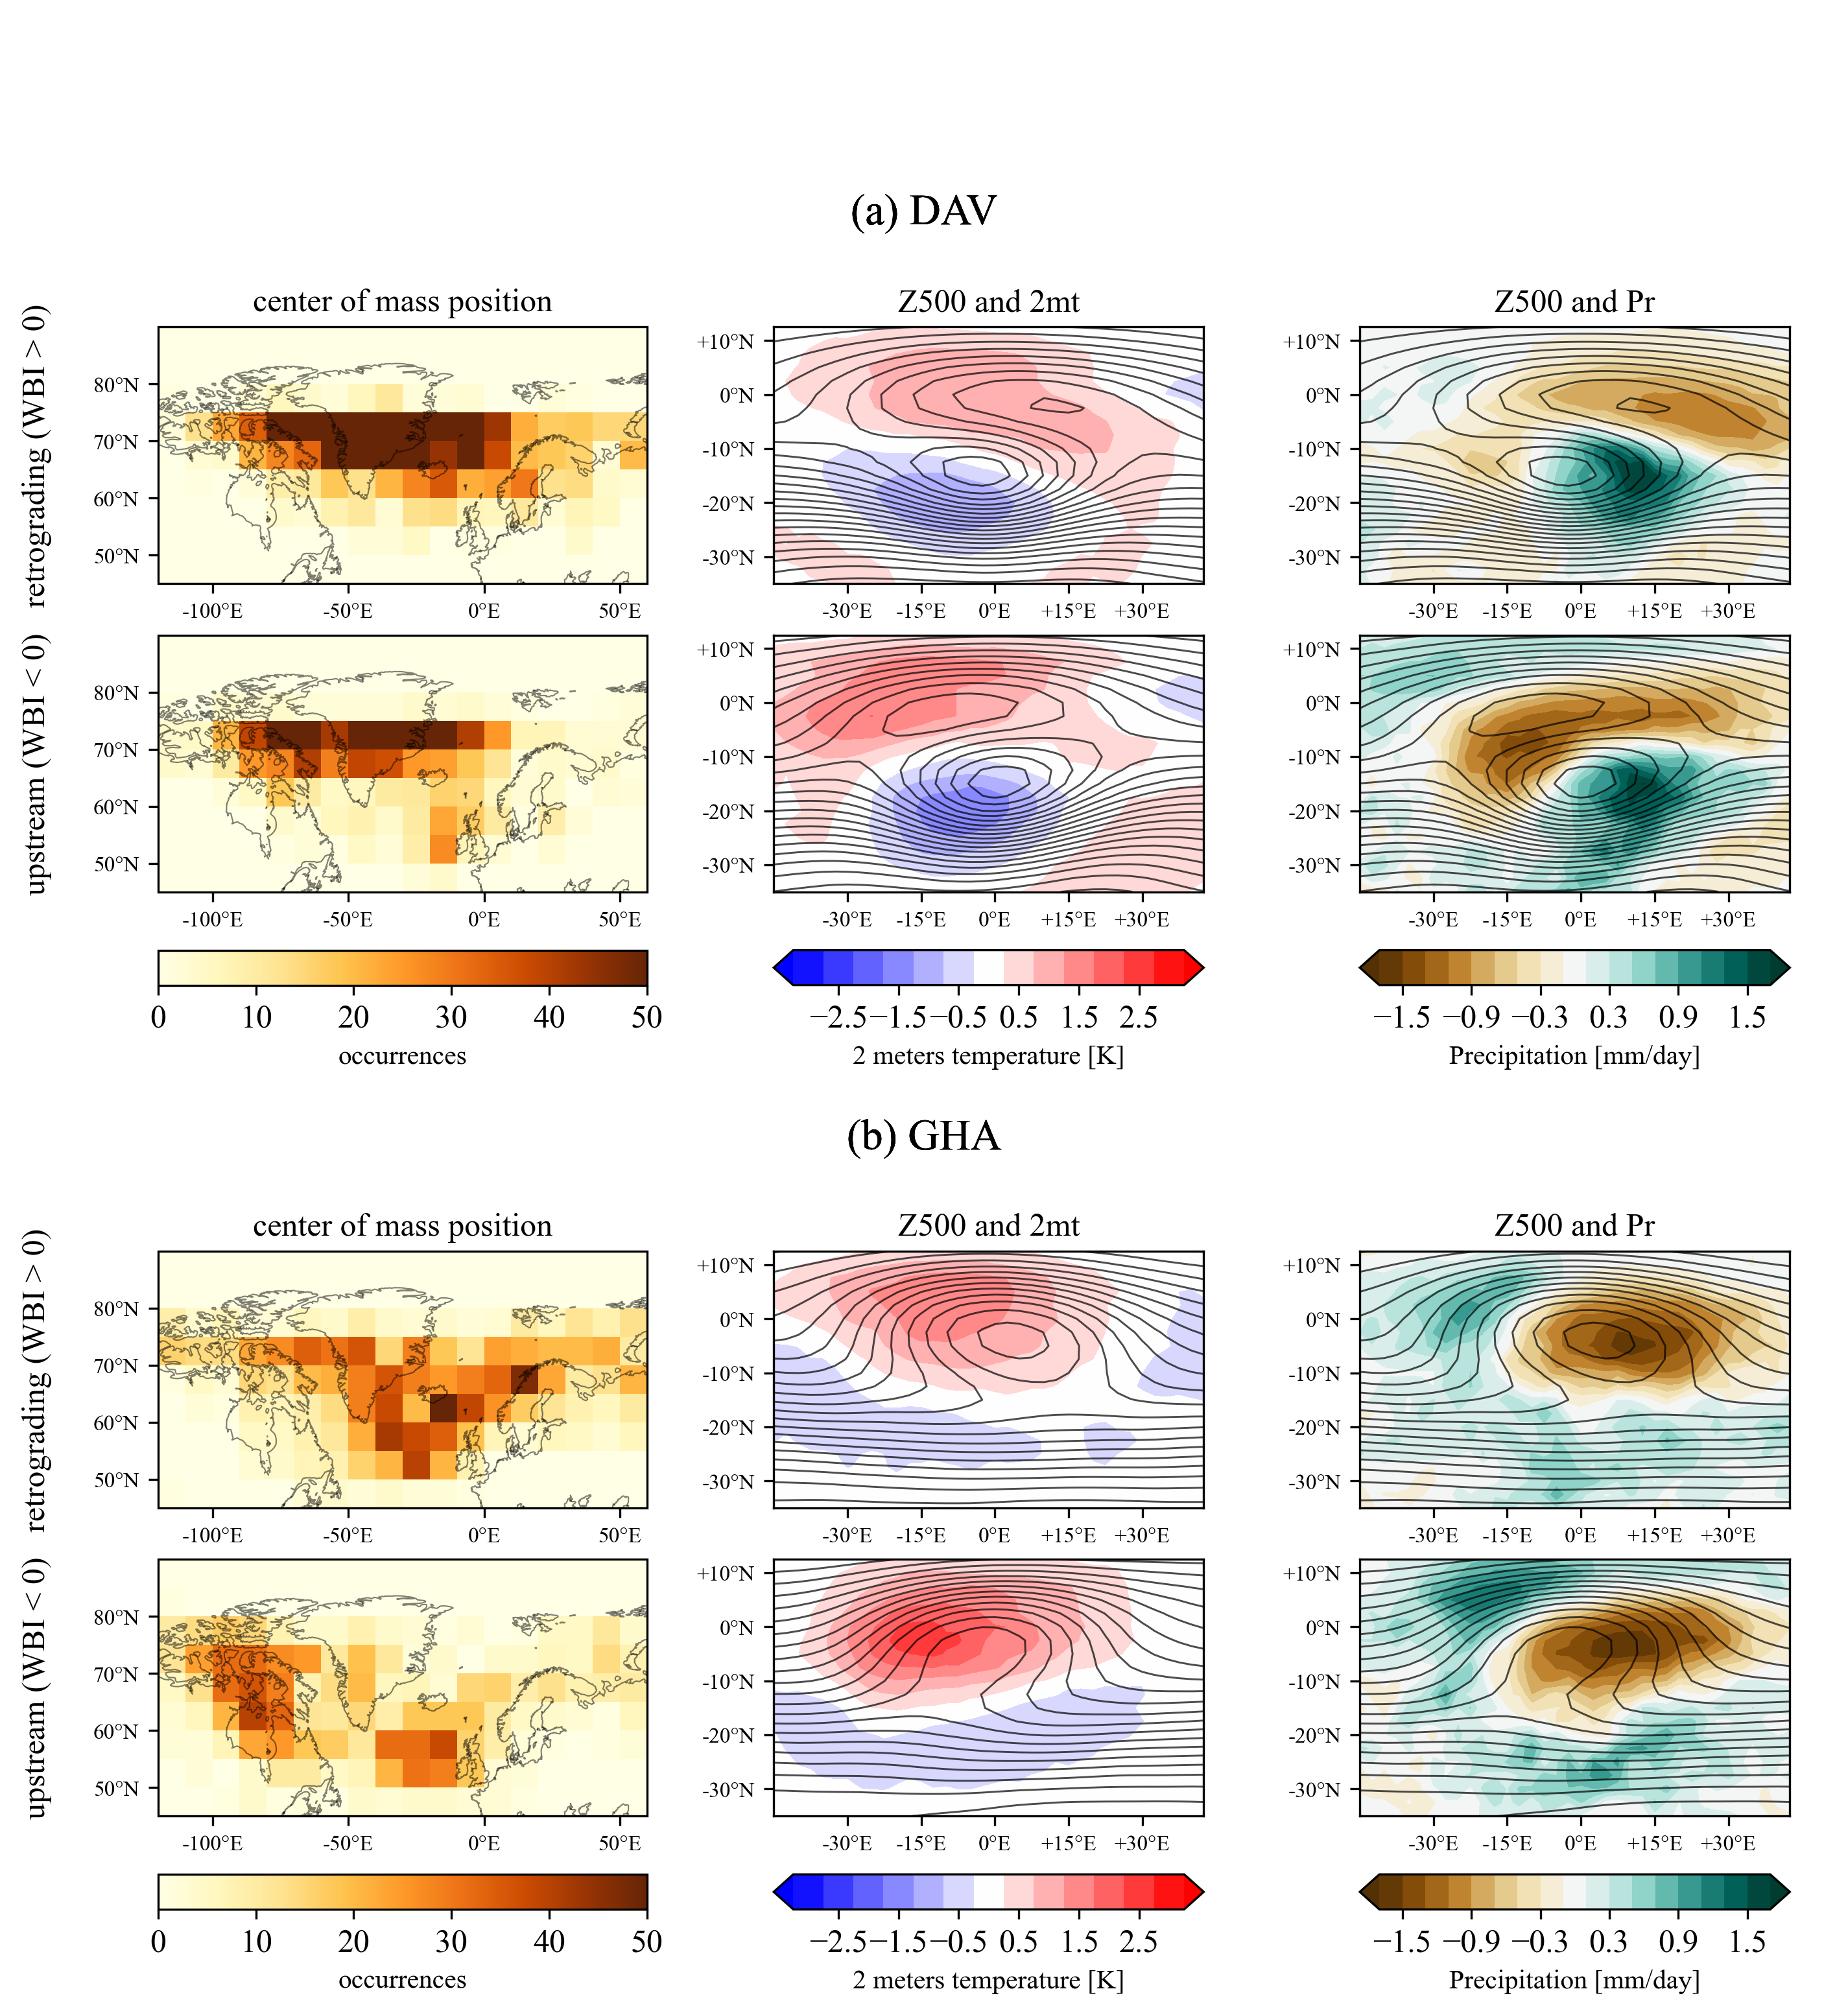} % Path to the image
    \caption{Composites and center of mass positions of retrograding and upstream blocking events over Greenland from ERA5 reanalysis (JJA). The center-of-mass position plots are 2D histograms with 10°lon × 5°lat bins, showing how often the center of mass of an upstream or retrograding block falls within each bin. Composite plots are plotted in the reference system of the block's center of mass (e.g. x axis represents relative longitude). Black contours represent the 500hPa geopotential height composite (Z500). Contours are plotted every $40 m$. Shadings refer to the composite anomaly of temperature above the surface (2 meters temperature - or 2mt \texttt{[} K \texttt{]}) and to the composite total precipitation. Anomalies have been computed with respect to the seasonal mean. A Student’s t-test was performed to assess the significance of the plotted anomalies, with all shaded contours significant at the 95\% confidence level. Panel a) showcases blocking events detected through the DAV index and panel b) showcases blocking events detected through the GHA index.}
    \label{composites_ERA5}
\end{figure}

\begin{figure}[htbp]
    \centering
    \includegraphics[width=\textwidth]{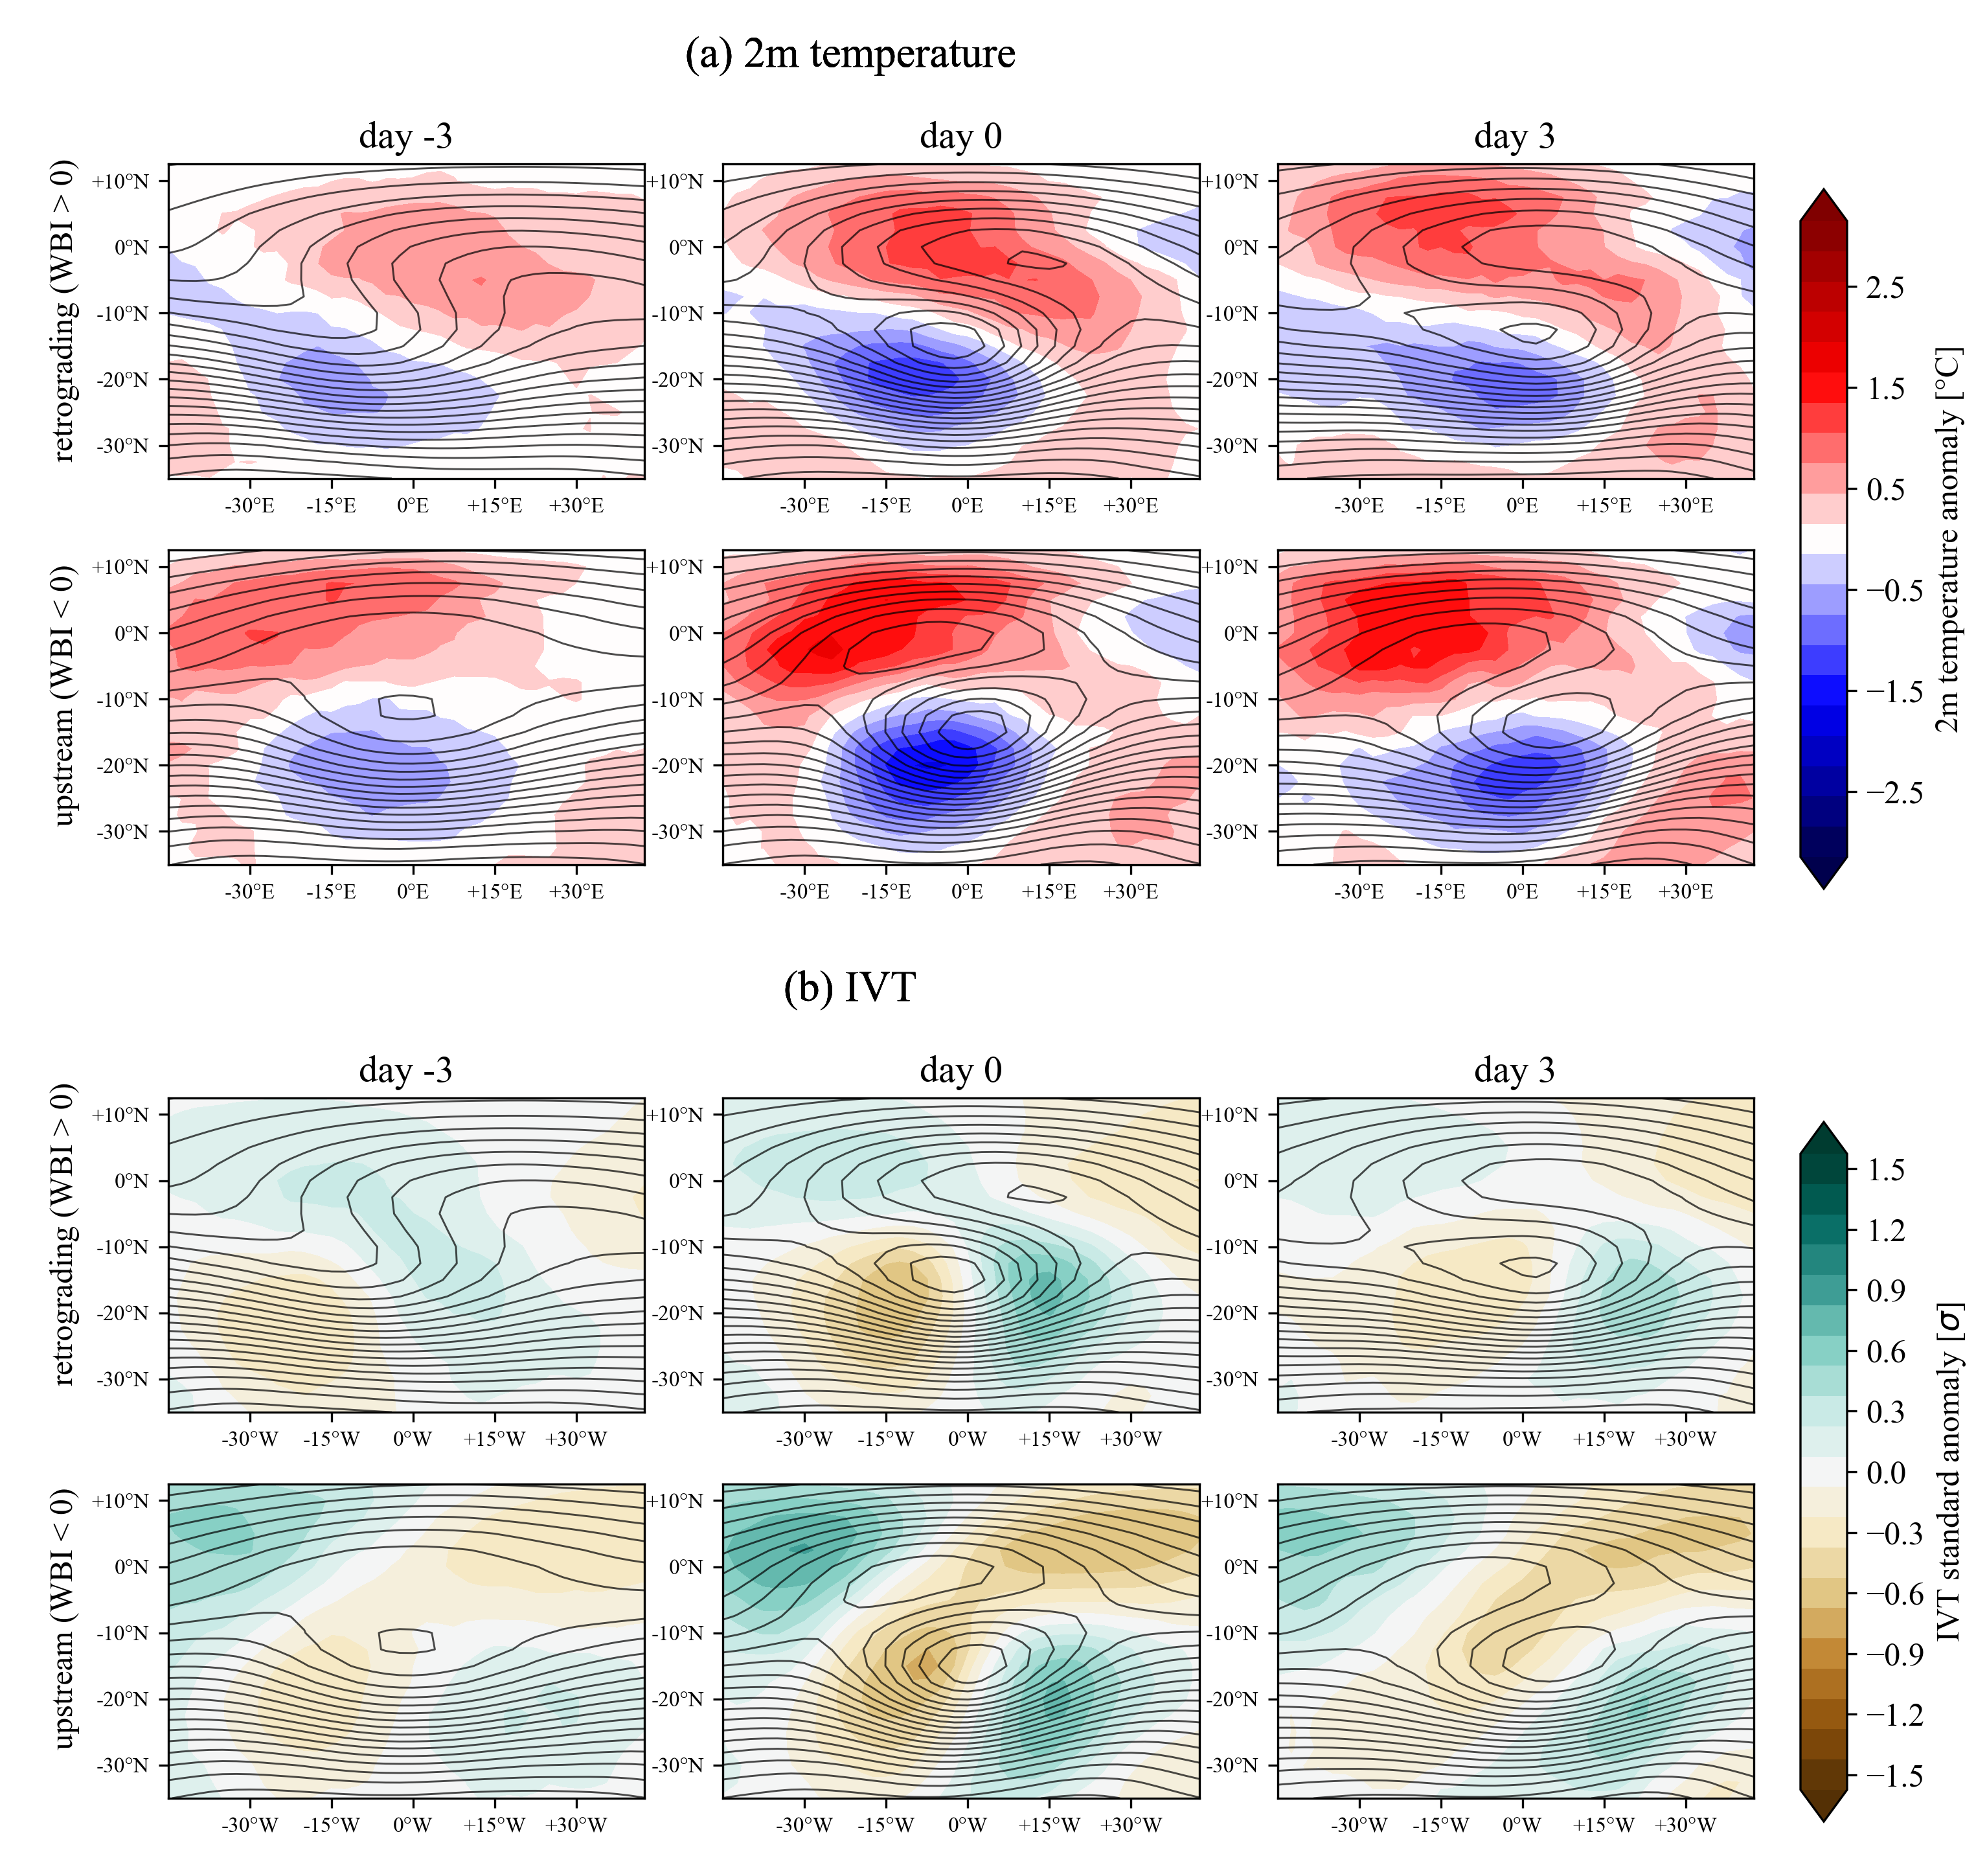}
    \caption{Composites of the time evolution of retrograding and upstream blocking events over Greenland from ERA5 reanalysis (JJA) detected through the DAV index. Composite plots are shown in the reference system of the block's center of mass. Black contours represent the 500~hPa geopotential height composite (Z500), plotted every 40~m. Shading refers to the composite anomaly of near-surface temperature (2~m temperature, K; panel A) and to the composite standardized anomaly of IVT (panel B). Anomalies are computed with respect to the seasonal mean. A Student’s \emph{t}-test was used to assess significance; all shaded regions are significant at the 95\% confidence level.}
    \label{fig:composites_time_evolv_dav}
\end{figure}

\begin{figure}[htbp]
    \centering
    \includegraphics[width=\textwidth]{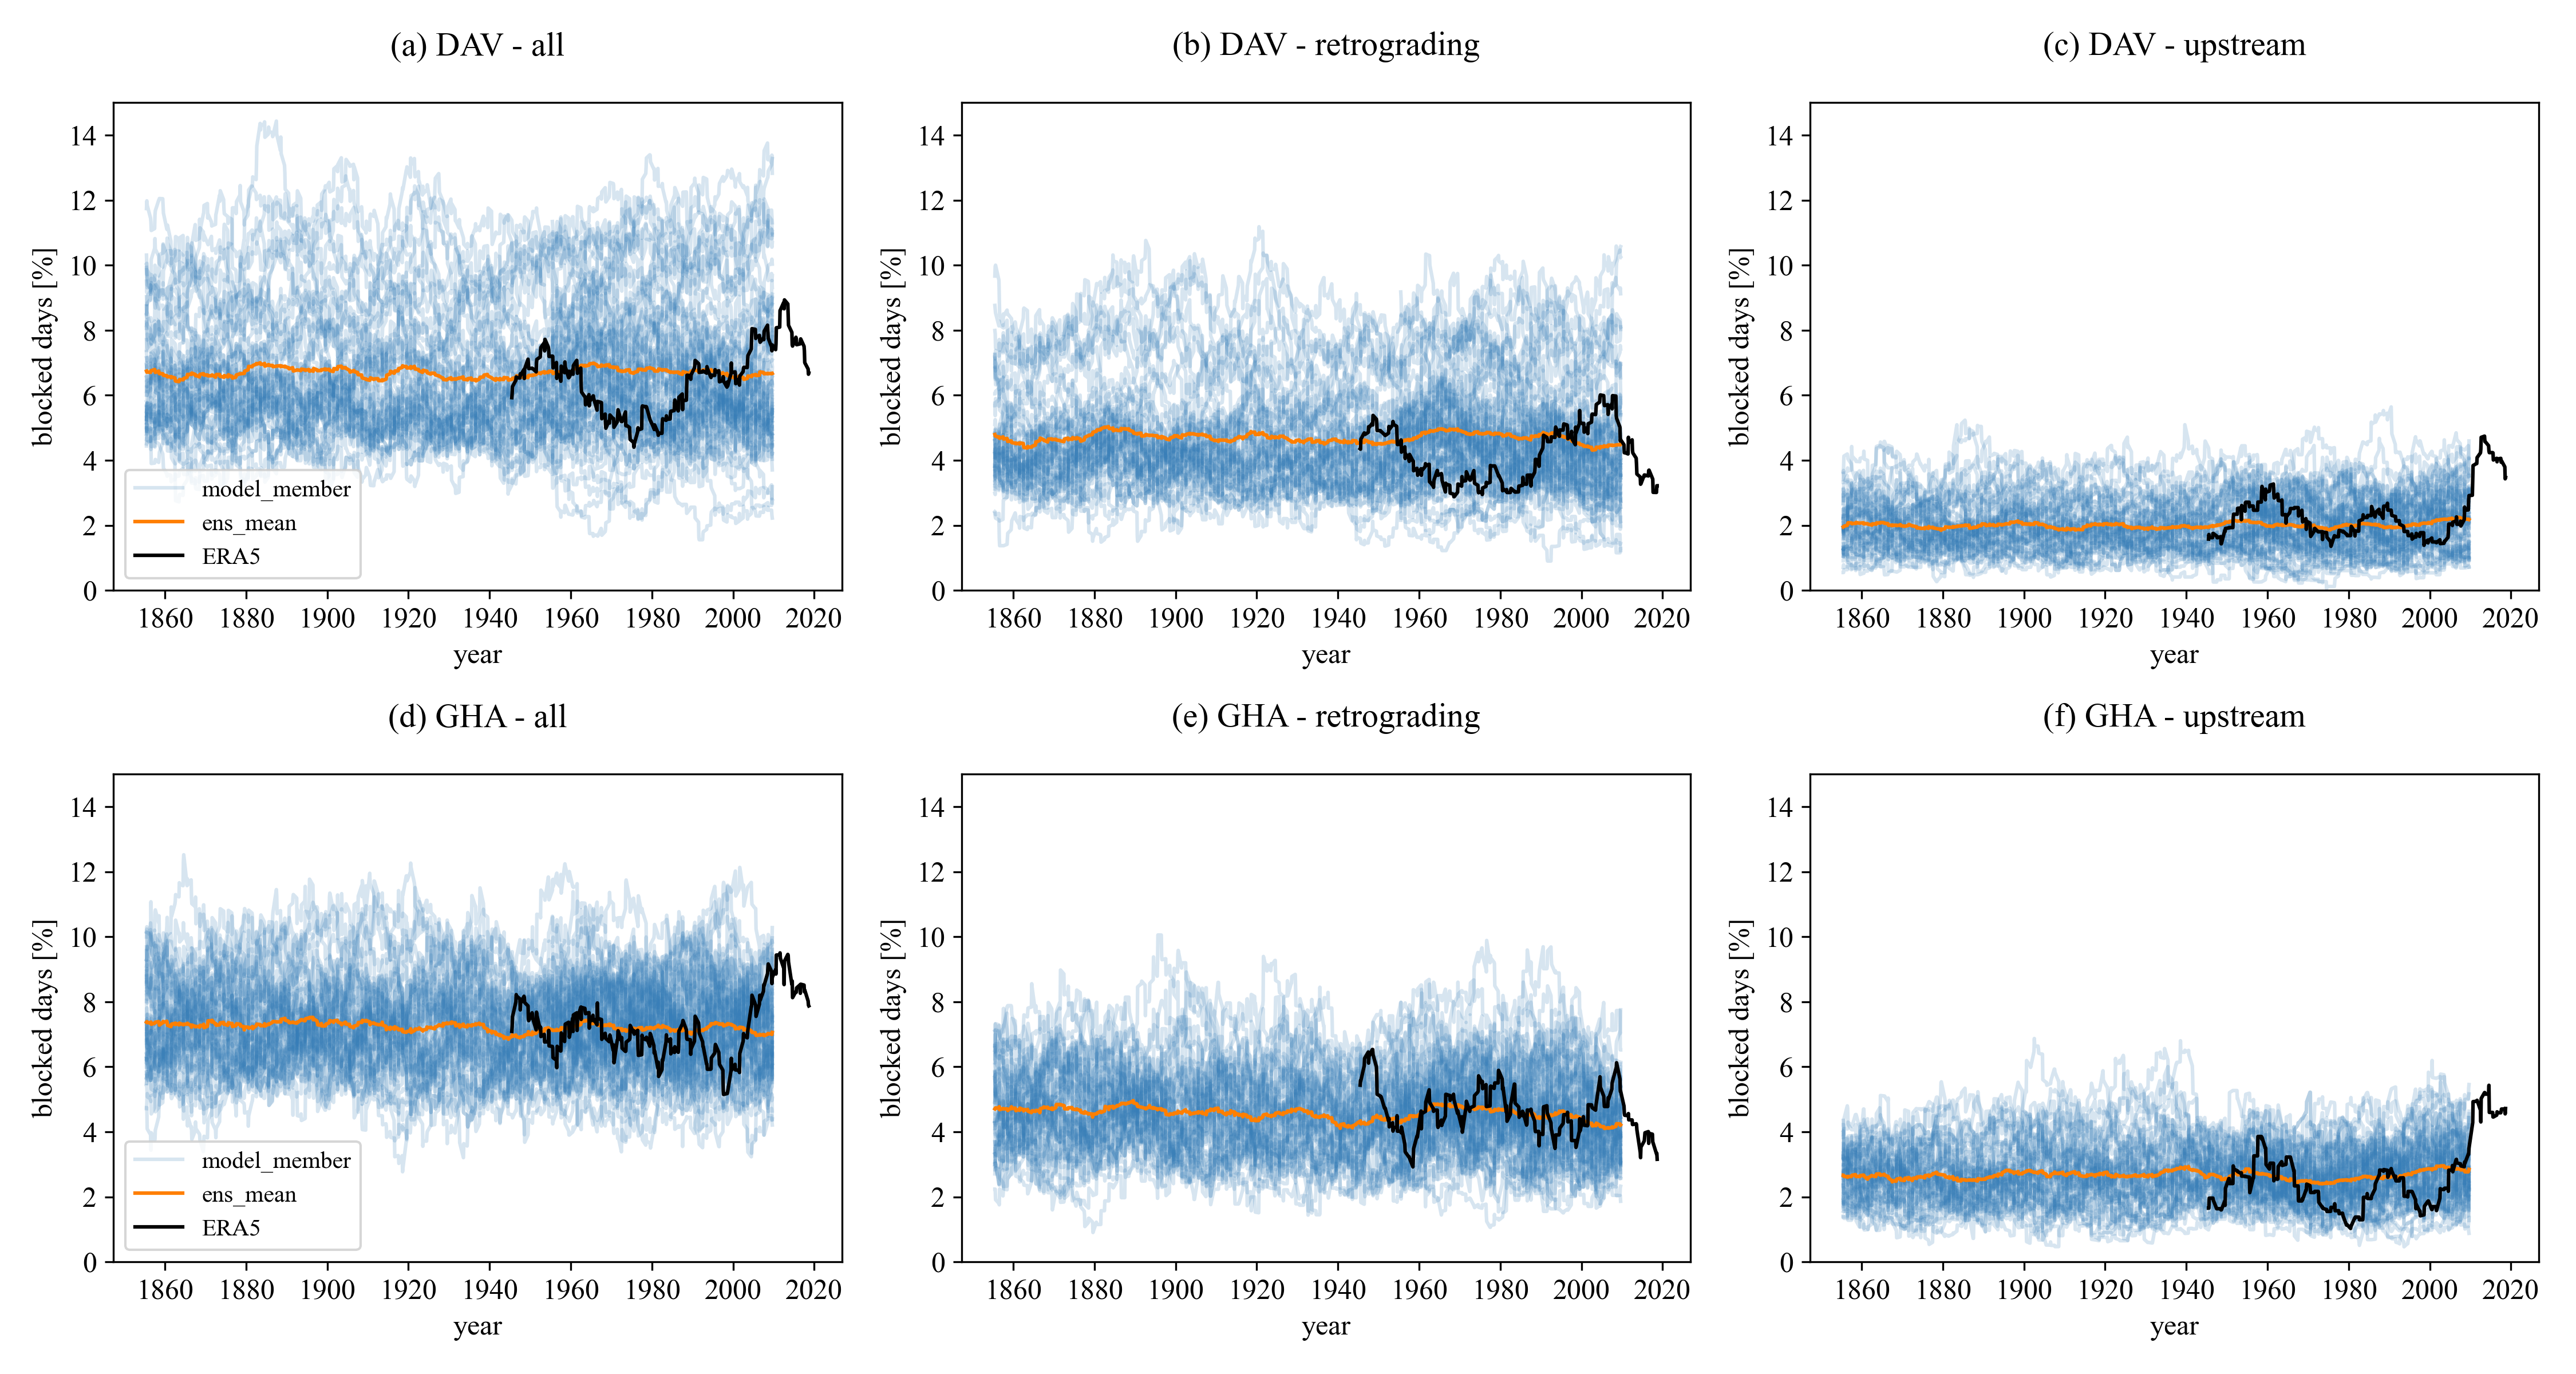}
    \caption{Summer (JJA) monthly blocking frequency time series. Black lines indicate ERA5 reanalysis, blue lines indicate individual CMIP6 ensemble members, and orange lines indicate the ensemble mean. The top row (a--c) shows blocking frequency detected using the DAV index, while the bottom row (d--f) shows frequency detected using the GHA index. The left column (a,d) refers to all blocking events crossing Greenland, the center column (b,e) to retrograding blocks, and the right column (c,f) to upstream blocks.}
    \label{fig:frequency_time_series}
\end{figure}

\begin{figure}[htbp]
    \centering
    \includegraphics[width=\textwidth]{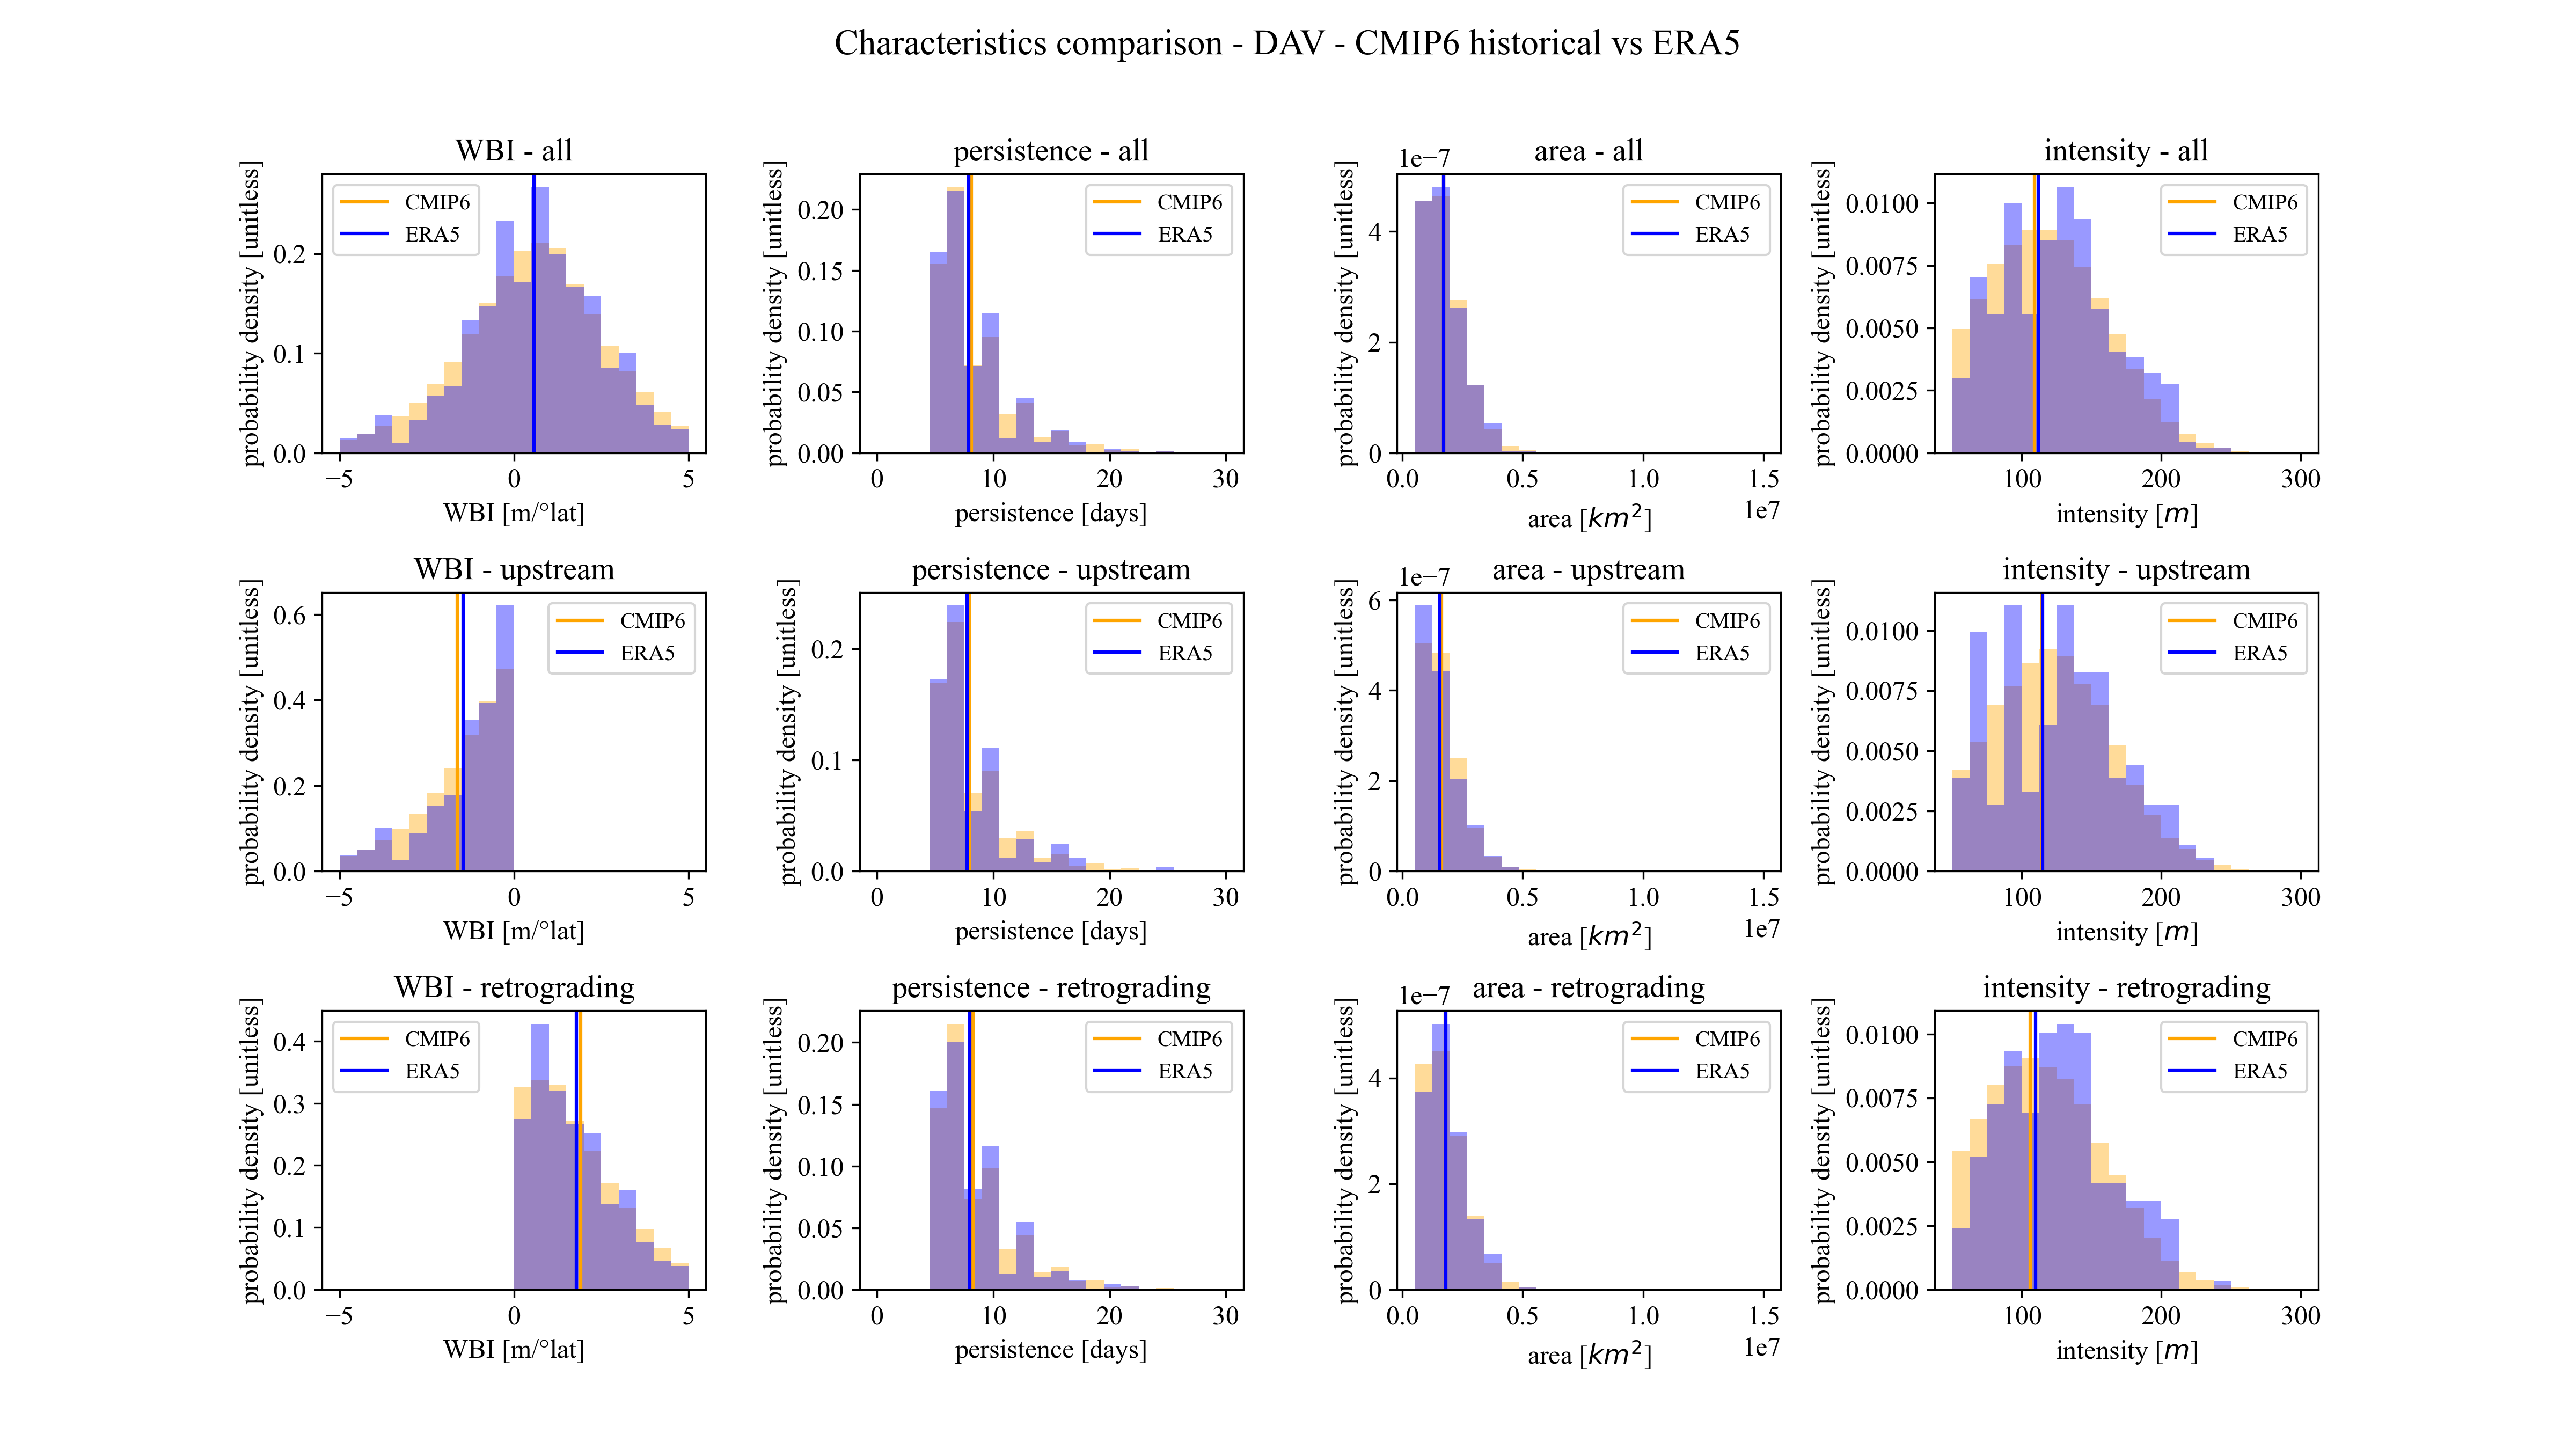}
    \caption{Comparison of blocking characteristics in ERA5 reanalysis and CMIP6 historical simulations detected using the DAV index. Rows correspond to different blocking types (top to bottom: all, upstream, and retrograding blocking events). Columns correspond to different characteristics (left to right: Wave Breaking Index, WBI, m/$^\circ$lat; persistence, days; area, km$^2$; and intensity, m). Purple indicates ERA5 and gold indicates the CMIP6 historical ensemble. Vertical lines denote distribution means.}
    \label{fig:char_dav_hist}
\end{figure}

\begin{figure}[htbp]
    \centering
    \includegraphics[width=\textwidth]{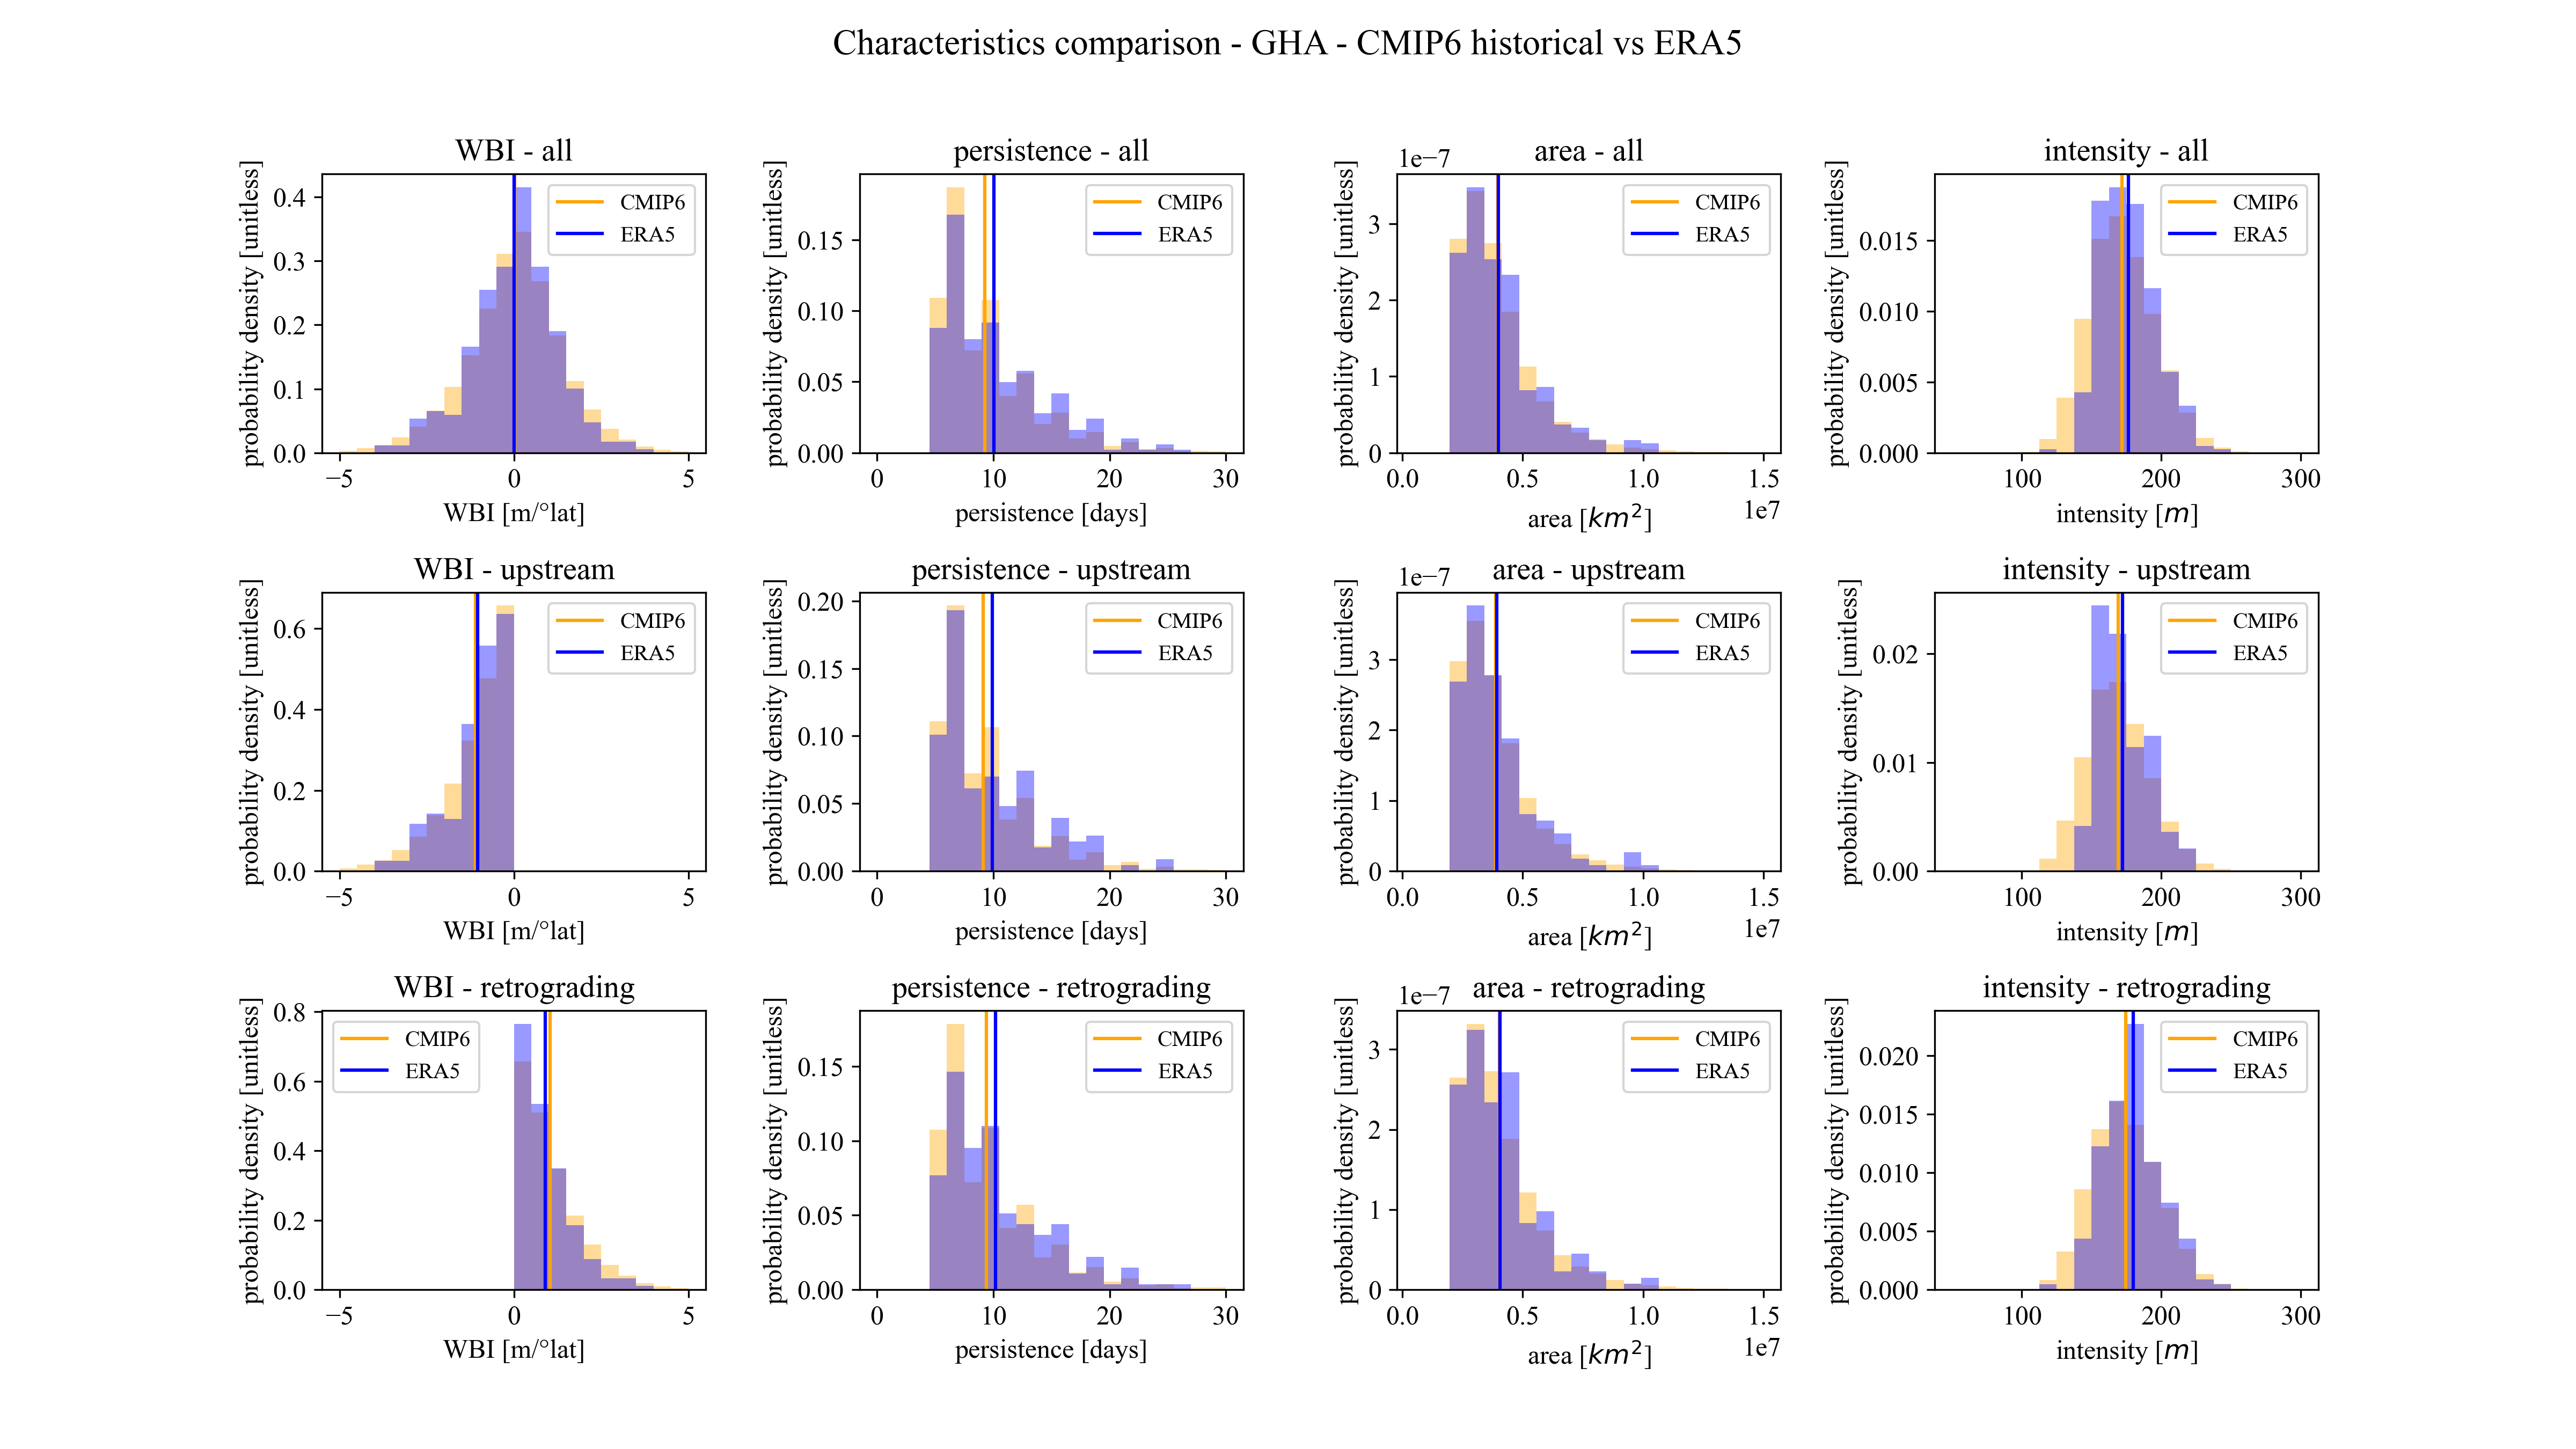}
    \caption{Same as Figure~\ref{fig:char_dav_hist}, but for blocking characteristics detected using the GHA index.}
    \label{fig:char_gha_hist}
\end{figure}

\begin{figure}[htbp]
    \centering
    \includegraphics[width=\textwidth]{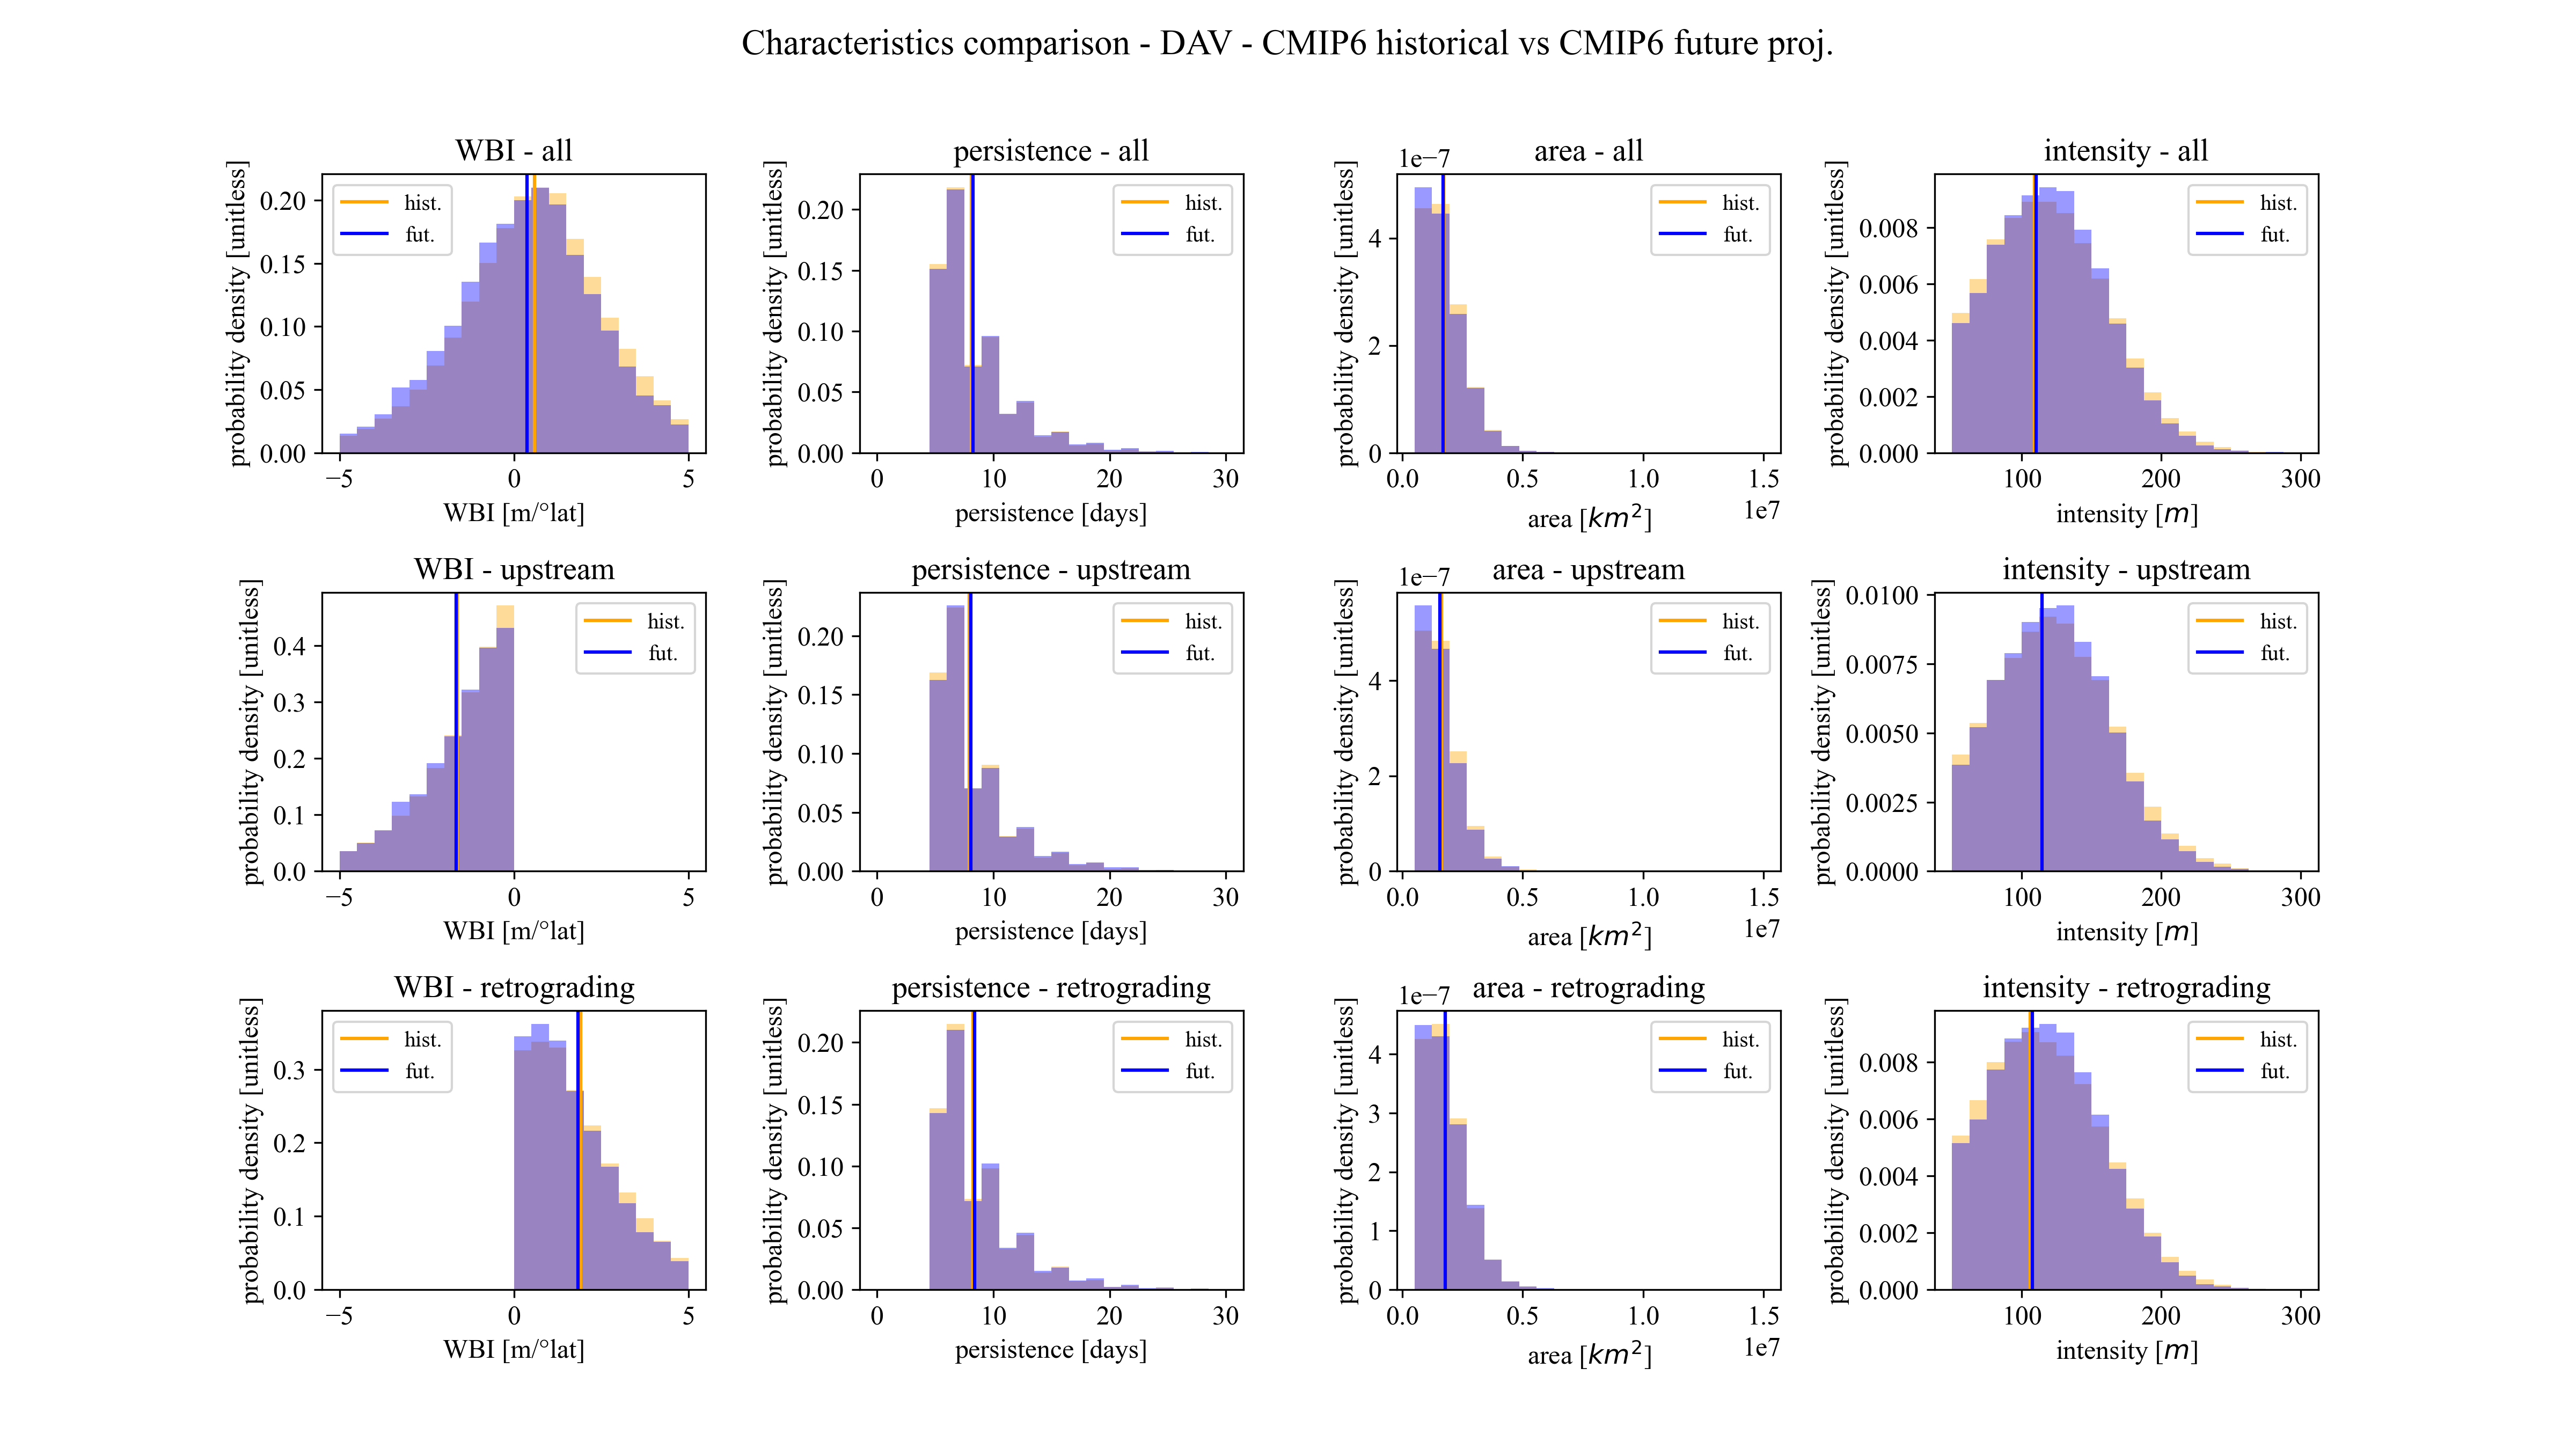}
    \caption{Comparison of blocking characteristics in CMIP6 historical simulations and CMIP6 future projections detected using the DAV index. Purple indicates the CMIP6 future ensemble and gold indicates the CMIP6 historical ensemble. Vertical lines denote distribution means.}
    \label{fig:char_dav_future}
\end{figure}

\begin{figure}[htbp]
    \centering
    \includegraphics[width=\textwidth]{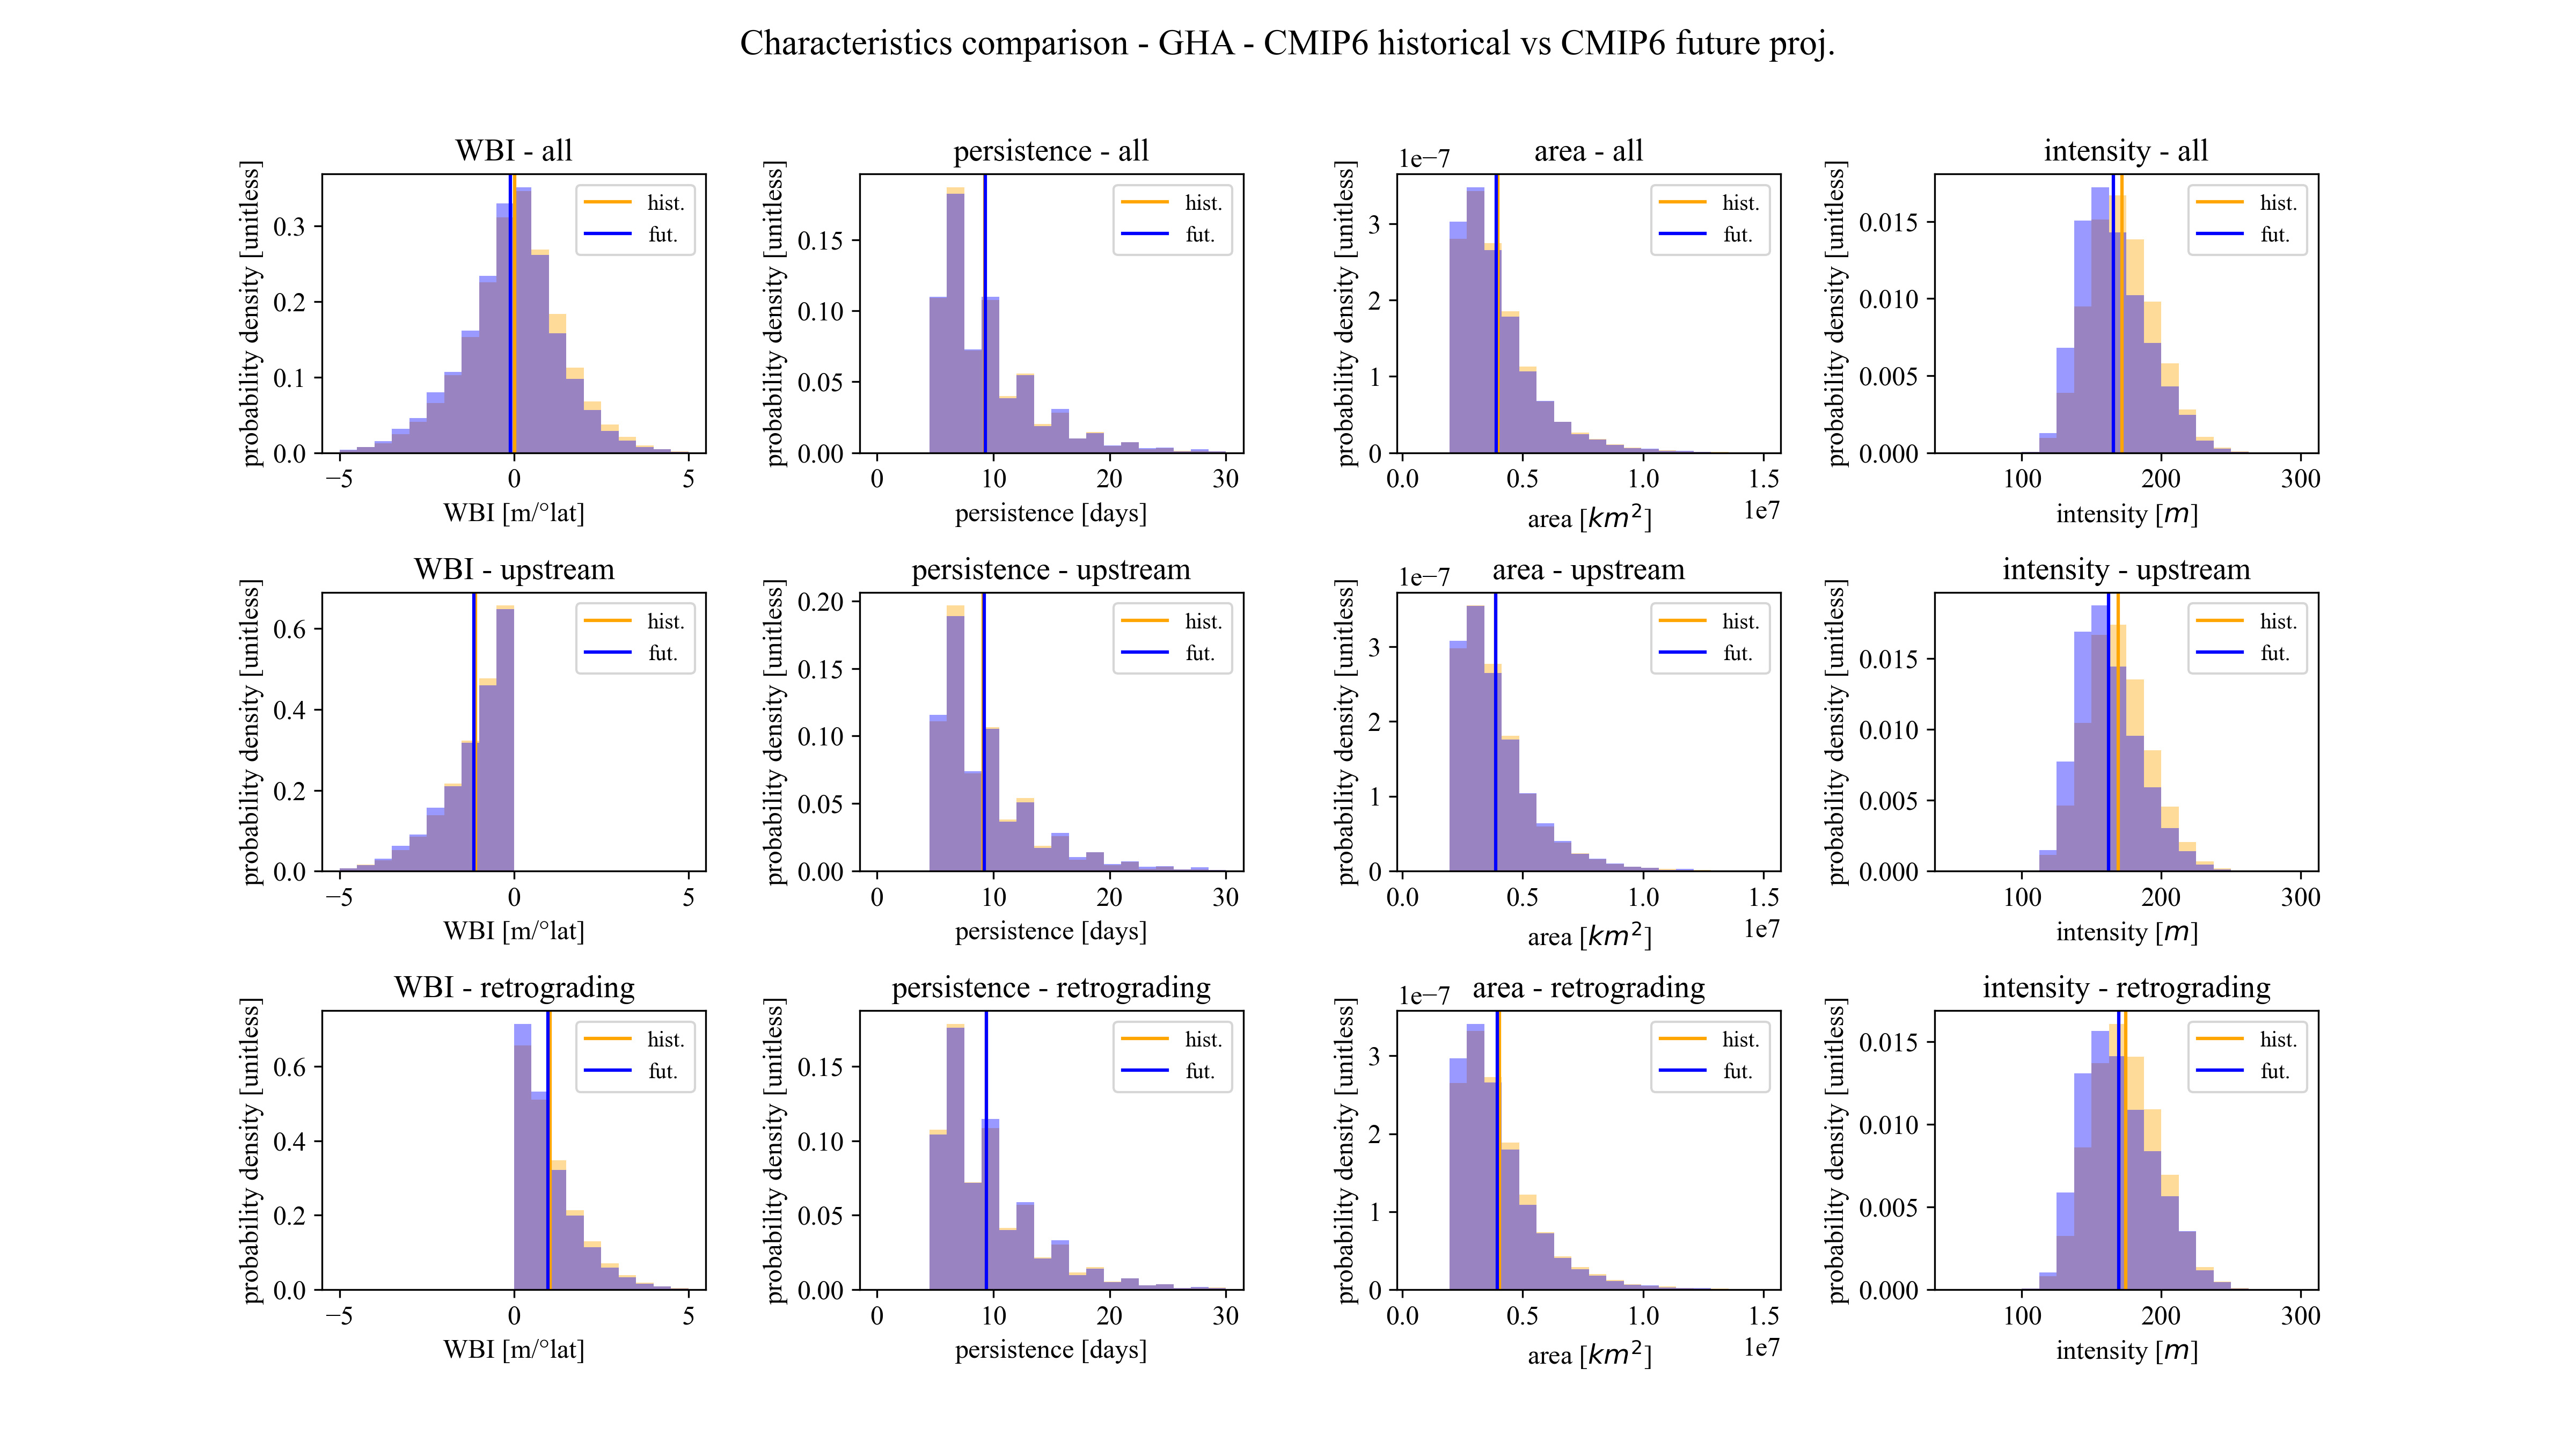}
    \caption{Same as Figure~\ref{fig:char_dav_future}, but for blocking characteristics detected using the GHA index.}
    \label{fig:char_gha_future}
\end{figure}

\end{document}
